# Supplementary material for: PolyDL: Polyhedral Optimizations for Creation of High Performance DL primitives
Source: arXiv:2006.02230 source file (2020-11-17)
Supplement: Supplementary file 1 [file appendix_txt.tex]

\section{Additional Experimental Results}

We use the PolyDL system to optimize the convolutions of  Xception (\textsf{xception}) \cite{DBLP:journals/corr/Chollet16a}, You Only Look Once v2 (\textsf{yolov2}) \cite{DBLP:journals/corr/RedmonDGF15}, 
MobileNets (\textsf{mobilenet}) \cite{DBLP:journals/corr/HowardZCKWWAA17},
AlexNet (\textsf{alexnet}) \cite{Krizhevsky:2012:ICD:2999134.2999257},
OverFeat (\textsf{overfeat}) \cite{sermanet2013overfeat}
GoogLeNet v1 and v3 \cite{43022},
and 
(\textsf{googlenetv1}, \textsf{googlenetv3}),
 the popular
and the state-of-the-art image recognition neural network models.
We also measure the performance of the same convolutions using 
the implementations from the Intel oneDNN library 
and those obtained via auto-tuning with the AutoTVM system.

\begin{figure*}[h!]
\centering
\begin{minipage}{0.49\textwidth}
\centering
\includegraphics[scale=0.25]{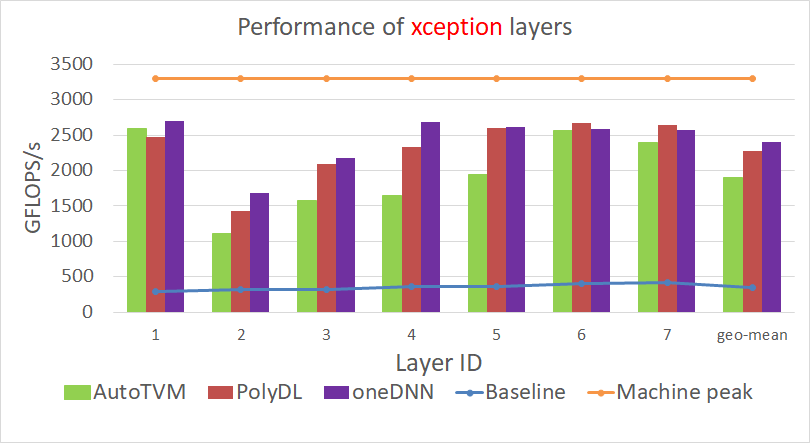}
\caption{Performance of xception layers}
\label{fig:xception}
\end{minipage}
\begin{minipage}{0.49\textwidth}
\centering
\includegraphics[scale=0.20]{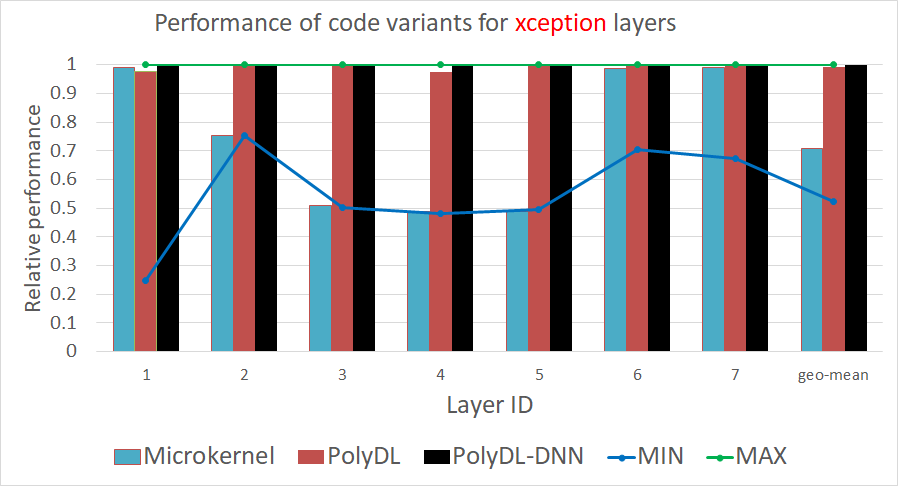}
\caption{Performance distribution of code variants}
\label{fig:xception_distro}
\end{minipage}
\end{figure*}

\begin{figure*}[h!]
\centering
\begin{minipage}{0.49\textwidth}
\centering
\includegraphics[scale=0.25]{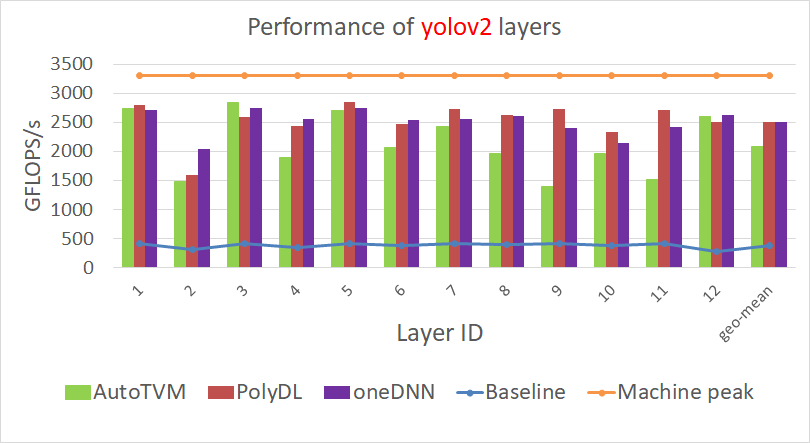}
\caption{Performance of yolov2 layers}
\label{fig:yolov2}
\end{minipage}
\begin{minipage}{0.49\textwidth}
\centering
\includegraphics[scale=0.2]{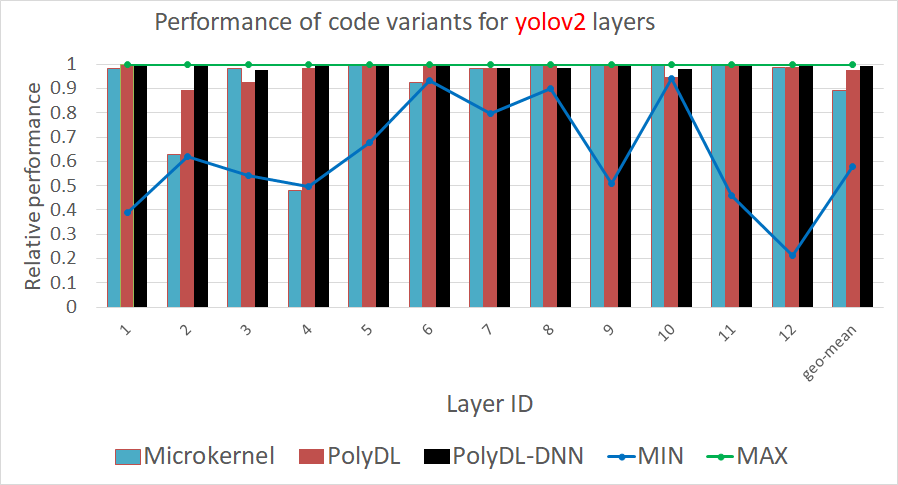}
\caption{Performance distribution of code variants}
\label{fig:yolov2_distro}
\end{minipage}
\end{figure*}

\begin{figure*}[h!]
\centering
\begin{minipage}{0.49\textwidth}
\centering
\includegraphics[scale=0.25]{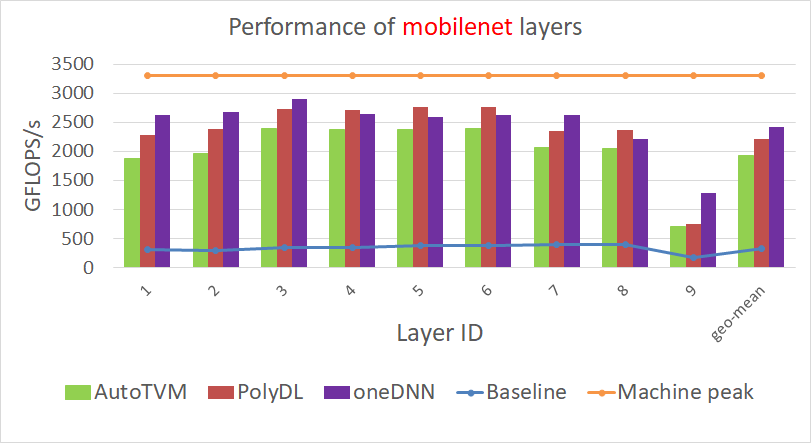}
\caption{Performance of mobilenet layers}
\label{fig:mobilenet}
\end{minipage}
\begin{minipage}{0.49\textwidth}
\centering
\includegraphics[scale=0.2]{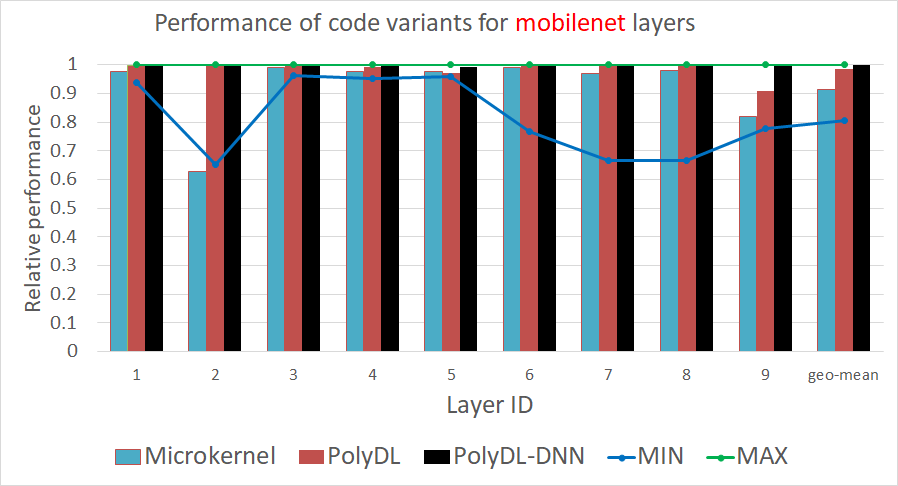}
\caption{Performance distribution of code variants}
\label{fig:mobilenet_distro}
\end{minipage}
\end{figure*}

\begin{figure*}[h!]
\centering
\begin{minipage}{0.49\textwidth}
\centering
\includegraphics[scale=0.25]{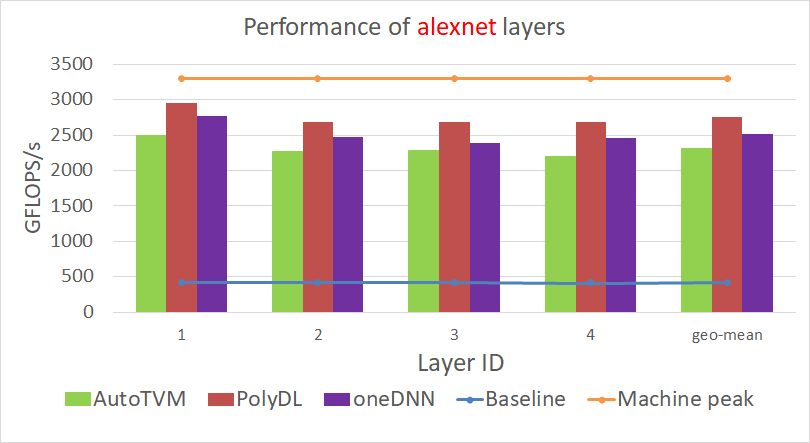}
\caption{Performance of alexnet layers}
\label{fig:alexnet}
\end{minipage}
\begin{minipage}{0.49\textwidth}
\centering
\includegraphics[scale=0.20]{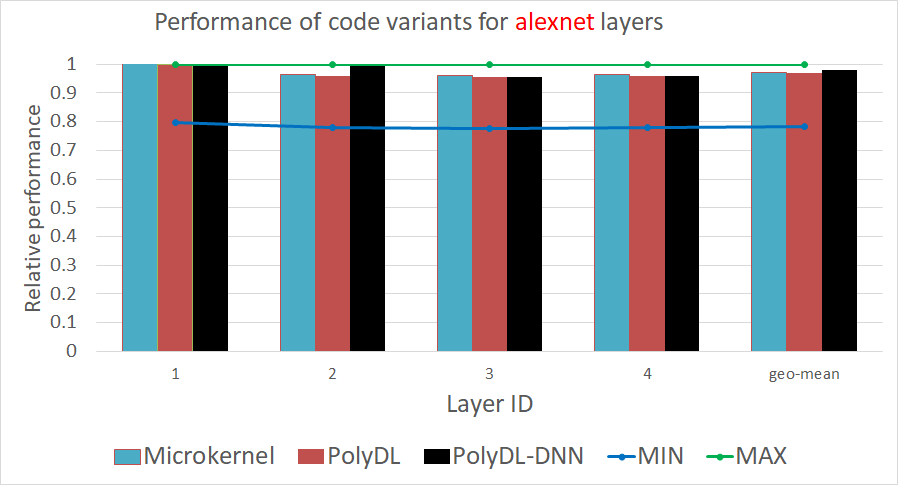}
\caption{Performance distribution of code variants}
\label{fig:alexnet_distro}
\end{minipage}
\end{figure*}

\begin{figure*}[h!]
\centering
\begin{minipage}{0.49\textwidth}
\centering
\includegraphics[scale=0.25]{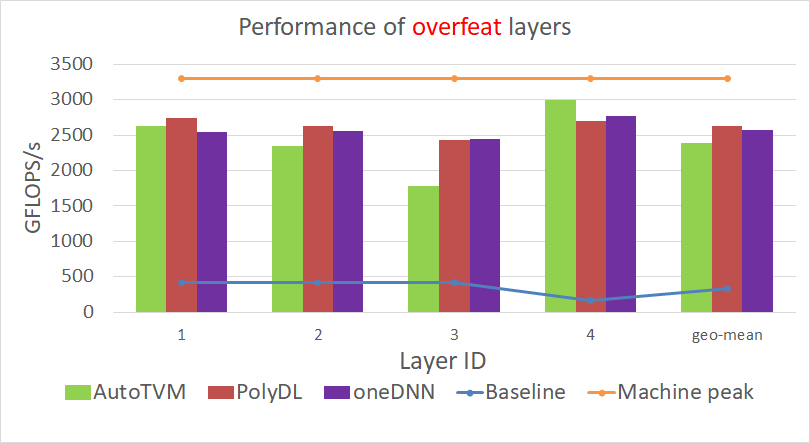}
\caption{Performance of overfeat layers}
\label{fig:overfeat}
\end{minipage}
\begin{minipage}{0.49\textwidth}
\centering
\includegraphics[scale=0.20]{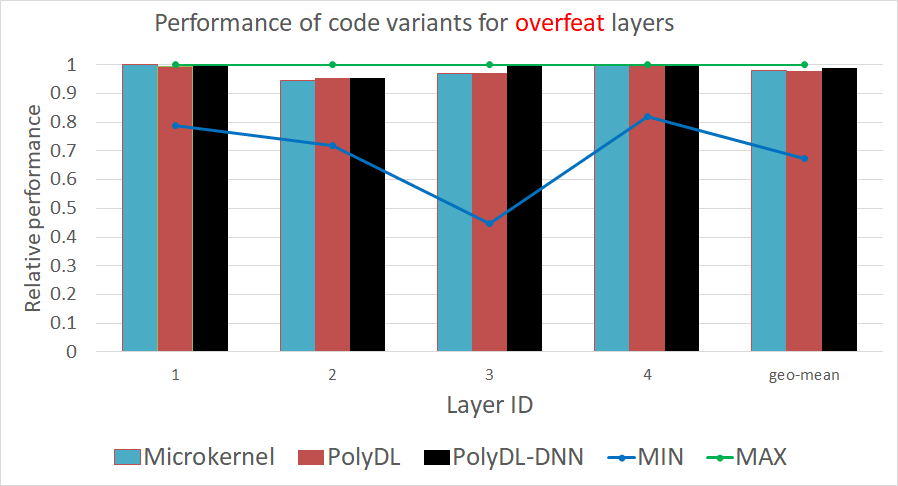}
\caption{Performance distribution of code variants}
\label{fig:overfeat_distro}
\end{minipage}
\end{figure*}

\begin{figure*}[h!]
\centering
\begin{minipage}{0.49\textwidth}
\centering
\includegraphics[scale=0.35]{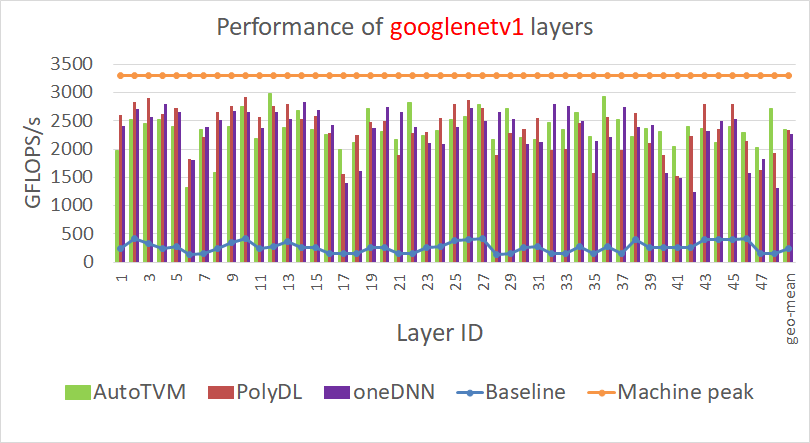}
\caption{Performance of googlenetv1 layers}
\label{fig:googlenetv1}
\end{minipage}
\begin{minipage}{0.49\textwidth}
\centering
\includegraphics[scale=0.30]{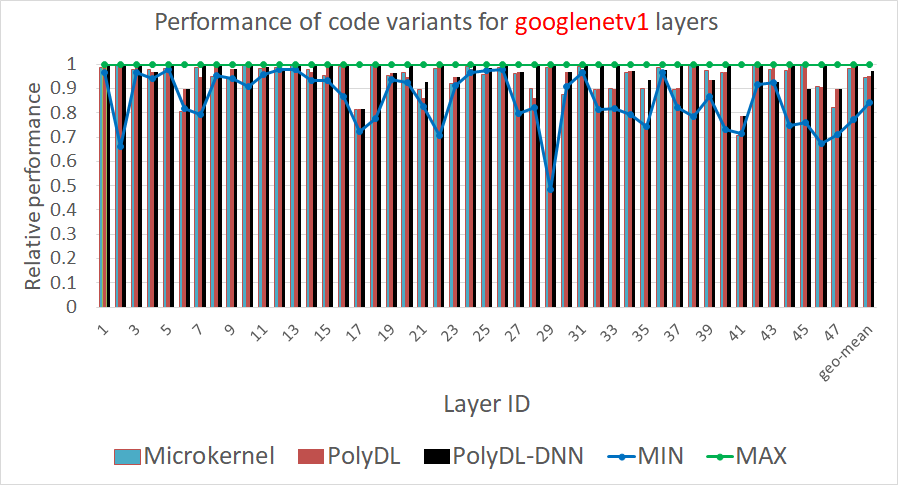}
\caption{Performance distribution of code variants}
\label{fig:googlenetv1_distro}
\end{minipage}
\end{figure*}

\begin{figure*}[h!]
\centering
\begin{minipage}{0.49\textwidth}
\centering
\includegraphics[scale=0.35]{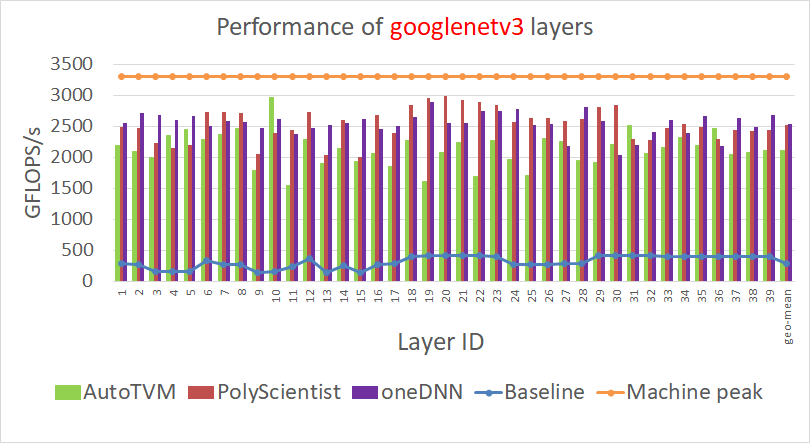}
\caption{Performance of googlenetv3 layers}
\label{fig:googlenetv3}
\end{minipage}
\begin{minipage}{0.49\textwidth}
\centering
\includegraphics[scale=0.30]{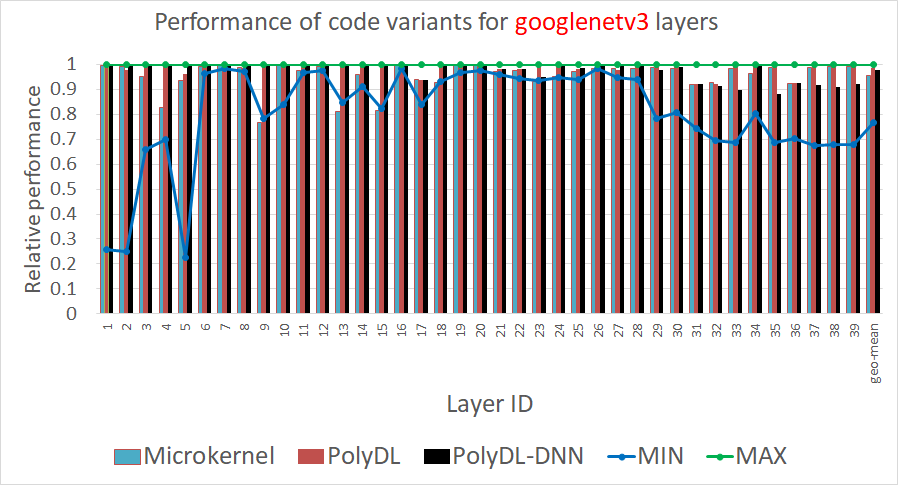}
\caption{Performance distribution of code variants}
\label{fig:googlenetv3_distro}
\end{minipage}
\end{figure*}

From Figure \ref{fig:xception} through Figure \ref{fig:googlenetv3_distro}, we show the performance
achieved by various systems and the performance distribution of code variants
seen for the CNN models, namely, \textsf{xception},
\textsf{yolov2}, \textsf{mobilenet}, \textsf{alexnet}, \textsf{overfeat},
\textsf{googlenetv1}, and finally \textsf{googlenetv3}.
In Figure \ref{fig:xception_distro}, we see that \textsf{PolyDL-DNN} picks the right 
variant for all layers of \textsf{xception}.
For \textsf{yolov2}  from Figure \ref{fig:yolov2}, we note that
PolyDL performance closely matches that of oneDNN. 
AutoTVM's performance lags behind that PolyDL's and oneDNN's.
Through Figure \ref{fig:yolov2_distro}, we see there is a great spread in 
performance of various code variants run.
In \textsf{mobilenet}, PolyDL consistently outperforms AutoTVM and on average is 1.14X faster 
(Figure \ref{fig:mobilenet}). Further, the different code variants 
perform very similarly for  for layers 1, 3, 4, and 5 in \textsf{mobilenet} while the performance spread
is greater for other layers (Figure \ref{fig:mobilenet_distro}).
In \textsf{alexnet}, PolyDL achieves superior performance compared to both AutoTVM and oneDNN for all layers (Figure \ref{fig:alexnet})
and on average is 1.19X and 1.09X faster than AutoTVM and oneDNN respectively.
In \textsf{overfeat}, PolyDL is slightly higher performing than oneDNN
and the performance spread is fair among different code variants generated
(Figures \ref{fig:overfeat}, and \ref{fig:overfeat_distro}).
\textsf{googlenetv1} and \textsf{googlenetv3} feature many more unique layers
and PolyDL's performance is slightly better than oneDNN's for 
\textsf{googlenetv1} and is slightly worse for \textsf{googlenetv3} 
(Figures \ref{fig:googlenetv1}, and \ref{fig:googlenetv3}).

PolyDL outperforms oneDNN in the case of  
\textsf{alexnet}, \textsf{overfeat}, and \textsf{googlenetv1}
and is significantly better than AutoTVM for all models except \textsf{googlenetv1}.
